# Supplementary material for: Toward responsible face datasets: modeling the distribution of a disentangled latent space for sampling face images from demographic groups
Source: arXiv:2309.08442 source file (2023-09-15)
Supplement: Supplementary file 1 [file appendix.tex]

\section{Appendix}

\subsection{A.1}
